# Supplementary material for: First Results for the pLGAD Sensor for Low-Penetrating Particles
Source: arXiv:2207.06047 source file (2022-07-19)
Supplement: Supplementary file 1 [file appendix.tex]

\subsection{Noise calculation}
\label{sec:noise_calculation}

For planar sensors at room temperature, the individual contributions to the Equivalent Noise Charge (ENC) are approximated as follows \cite{BERGAUERPHD}:

\begin{align}
	\label{eq:noise_approximation}
	&\ENC_C &= a + b \cdot \mathit{ENF} \cdot C  \\
	&\ENC_J &\approx 107 \sqrt{\Jleak \cdot \tint} \\
	&{\ENC}_{\RP}    &\approx 772 \sqrt{\frac{\tint}{\RP}} \\
	&{\ENC}_{\RS}    &\approx 0.395 \cdot C \cdot \sqrt{\frac{\RS}{\tint}}.
\end{align}

The capacitive load $C = \Cint + \Cback$ is the sum of the capacitance between the sensing elements \Cint{} and the \gls{cback} \Cback{}.
$a$ and $b$ are constants depending on the readout chip. 
\Jleak{} denotes the \gls{dark current} in \si{\nano\ampere}, and \tint{} is the integration time of the readout chip in \si{\micro\second}.
\RP{} is the parallel resistor in \si{\mega\ohm} and \RS{} is the series line resistor in \si{\ohm}. It should be noted that pixelated sensors usually don't have dedicated bias resistors like \glspl{sms} do. So, for pixelated sensors the parallel resistor is defined by the inter-pixel resistance, which usually is very high.
The excess noise factor $\mathit{ENF}$ increases the shot noise in semiconductor devices with internal amplification, which applies to the series component of the capacitive noise.
In our case, it amounts to $\mathit{ENF} = 2.9$, calculated according to \cite{DALLABETTA2015}.

Under the justified assumption that the aforementioned noise sources are uncorrelated, the total noise is calculated as:

\begin{equation}
	\ENC^2 = \ENC_\mathrm{C}^2 + \ENC_\mathrm{J}^2 + {\ENC}_{\RP}^2 + {\ENC}_{\RS}^2.
\end{equation}

The minimum number of detectable primary \glspl{ehpair} is calculated from the desired Signal to Noise Ratio (SNR) and the gain as: 

\begin{equation}
	\label{eq:detection_threshold}
	\begin{aligned}
	p_\mathrm{min} &= \ENC \cdot SNR/\mathrm{gain}\\ 
	&=\ENC / 2 ~\mathrm{for} ~SNR = 5, \mathrm{gain} = 10
	\end{aligned}
\end{equation}

Usually, the required SNR is set to 5, to obtain a 5-sigma significance of the detection. The gain of 10 is a reasonable assumption of the expected gain of a pLGAD sensor.

\begin{table*}[htb]
	\label{tab:noise_parameters}
	\centering
	\begin{tabular}{rlll}
		\toprule
		Parameters & Single channel & NoMoS & Timepix3 \\
		\midrule
		Readout system 	& AliVata 	& Timepix3 	& Timepix3 \\
		Design parameters of (pre)-amplifier $a$, $b$				& 70, 12 		& 62, 0~\cite{PITTERS2018} 		& 62, 0 \\
		Integration Time \tint{} (\si{\micro\second}) & 0.05 & 0.05 & 0.05 \\
		\midrule
		Parallel Resistor \RP{} (\si{\mega\ohm}) & 100  & 100 & 100\\
		Series Resistor \RS{} (\si{\ohm}) & 10  & 10 & 10\\
		\midrule
		Pixel size (\si{\micro\metre\squared}) & $3000 \times 3300$ & $400 \times 1600$ & $55 \times 55$ \\
		Capacitive load $C$ (\si{\pico\farad}) & 3.5 & 0.066 & 0.001 \\
		Sensor thickness (\si{\micro\metre}) & 320 & 1000 & 320 \\
		Leakage current (\si{\nano\ampere\per\cubic\milli\metre}) & 1.1 & 1.1 & 1.1 \\
		Gain  & 10 & 10 & 10 \\
		\bottomrule
	\end{tabular}
	\caption{Parameters and their (assumed) values for the noise estimations. The first section shows the parameters of the readout systems, the second section gives assumptions about the connection to the sensor, and the third section shows the parameters of the sensor itself. For more information refer to \cref{sec:noise_calculation}}
\end{table*}

\subsection{Calculation of the detection efficiency}
\label{sec:detection_efficiency}

In order to determine the efficiency of the sensor, first 50,000 protons impinging normal to a silicon detector with \SI{15}{\nano\meter} of aluminium passivization layer for a specific energy were simulated using IMSIL \cite{hobler_monte_1995}. Afterwards, individual proton tracks were followed and the electronic energy loss deposited per step was extracted as a function of position. This histogram was then convoluted with the energy required to free an \gls{ehpair} in silicon and the best case CCE (see \cref{fig:entrance_window} top) for each proton. The results were sorted into a histogram which represents a distribution of the \glspl{ehpair} created within the sensor such as those shown in \cref{fig:histogram_imsil15} for $10$ and \SI{15}{\kilo\electronvolt} energy of the impinging protons. From this histogram, an efficiency plot is generated by summing over the number of protons starting from a specific \gls{ehpair} to the total \gls{ehpair} $n$ and then dividing the value by the total number of simulated protons $N=50,000$ i.e.
\begin{equation}
\varepsilon_{p_{k}}=\dfrac{1}{N}\sum\limits_{j=i}^{n}\#_j\quad \textrm{where}\quad i=2,3,4,\dots,n-1
\label{eq:binSummation}
\end{equation}
Note that the definition range of $i$ starts from 2 as the first bin contains the number of protons that did not reach the active area of the detector. This gives us the percentage of protons which generate a specific number of \glspl{ehpair}.
\begin{figure*}[h]
	\centering
	\includegraphics[width=\linewidth]{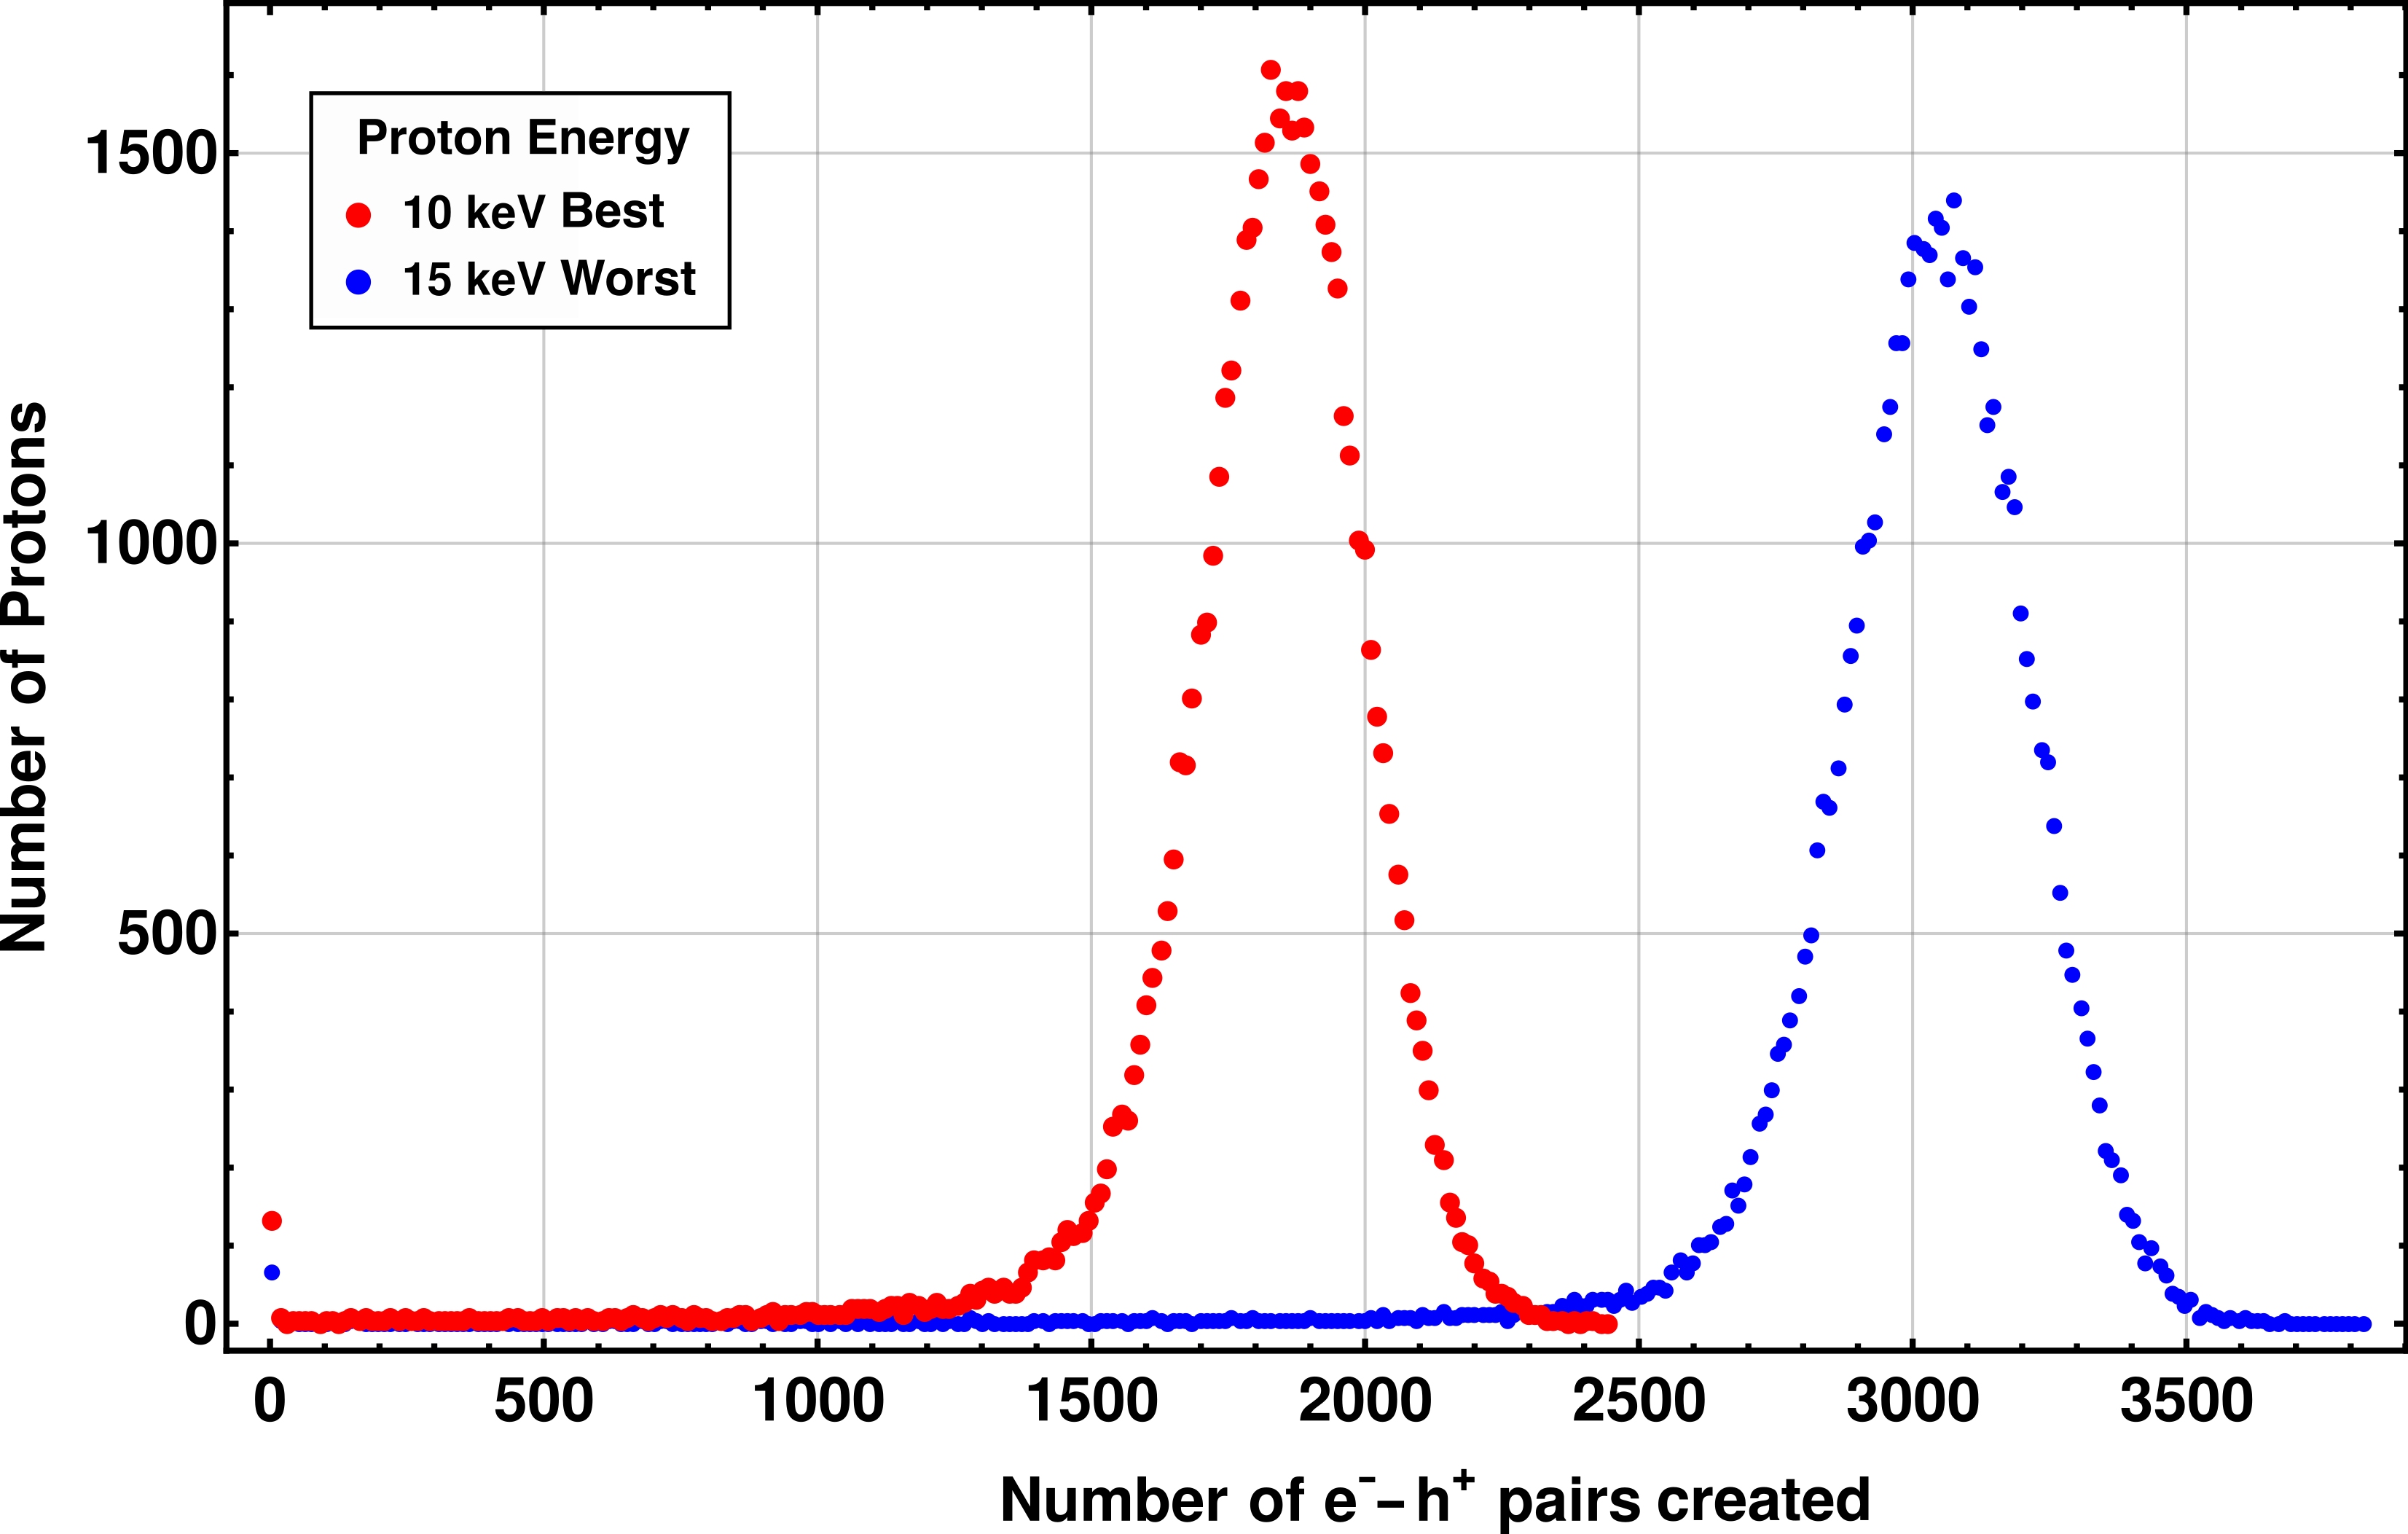}
	\caption{Histogram showing the number of protons as a function of the number of electron hole (e-h) pairs created within the pLGAD sensor by protons impinging on the sensor normal to the sensor surface with 10 and \SI{15}{\kilo\electronvolt}. The two histograms show the convolution of CCE in the best and worst case scenarios (cf. \cref{fig:entrance_window}). The entry at $0\,\glspl{ehpair}$ represents the protons that did not reach the active layer of the sensor and were either absorbed or backscattered from the passivation layer.}
	\label{fig:histogram_imsil15}
\end{figure*}
